# Supplementary material for: Spectropolarimetry of stripped envelope core collapse supernovae and their progenitors
Source: arXiv:1906.07184 source file (2019-06-17)
Supplement: Supplementary file 1 [file AppendixTemplate.tex]

%Appenndix for line measurements in IRTF + other spectra

%\label{app:line_measure}

\chapter{Infra-red line measurements}
\label{app:line_measure}

\lhead{\emph{IR line measurements}}

%==============================================================================
%optional contents
{\Large \textbf{Contents} }\\


%==============================================================================
